# Supplementary material for: Rethinking electrified transportation: The case for dynamic wireless charging
Source: arXiv:2610.18708 source file (2026-10-26)
Supplement: Supplementary file 1 [file Supplementary_main.tex]

% Compatibility wrapper; select the root-level Supplementary_main.tex.
\input{Supplementary_main.tex}
